# Supplementary material for: DeepCloak: Adversarial Crafting As a Defensive Measure to Cloak Processes
Source: arXiv:1808.01352 source file (2020-04-23)
Supplement: Supplementary file 1 [file appendix.tex]

\appendix
\section{Appendix}

\subsection{Classical ML Methods}\label{app:classical_ml}

The following is the full list of the classical ML methods used in the study.

\begin{itemize}[noitemsep]
	\item Fine Tree
	\item Medium Tree
	\item Coarse Tree
	\item Linear Discriminant
	\item Quadratic Discriminant
	\item Linear SVM
	\item Quadratic SVM
	\item Cubic SVM
	\item Fine Gaussian SVM
	\item Medium Gaussian SVM
	\item Coarse Gaussian SVM
	\item Fine kNN
	\item Medium kNN
	\item Coarse kNN
	\item Cosine kNN
	\item Cubic kNN
	\item Weighted kNN
	\item Boosted Trees
	\item Bagged Trees
	\item Subspace Discriminant
	\item Subspace kNN
	\item RUSBoosted Trees
\end{itemize}

The following descriptions about the classifiers are taken from Mathworks webpage~\cite{mathworks_classifiers}.

\textbf{Decision Tree:} are easy to interpret, fast for fitting and prediction, and low on memory usage, but they can have low predictive accuracy. Try to grow simpler trees to prevent overfitting. Control the depth with the Maximum number of splits setting.

\textbf{Discriminant Analysis:} is a popular first classification algorithm to try because it is fast, accurate and easy to interpret. Discriminant analysis is good for wide datasets. Discriminant analysis assumes that different classes generate data based on different Gaussian distributions. To train a classifier, the fitting function estimates the parameters of a Gaussian distribution for each class.

\textbf{SVM:} classifies data by finding the best hyperplane that separates data points of one class from those of the other class. The best hyperplane for an SVM means the one with the largest margin between the two classes. Margin means the maximal width of the slab parallel to the hyperplane that has no interior data points.

\textbf{kNN:} typically have good predictive accuracy in low dimensions, but might not in high dimensions. They have high memory usage, and are not easy to interpret. kNN classification is basically categorizing query points based on their distance to points (or neighbors) in a training dataset can be a simple yet effective way of classifying new points. You can use various metrics to determine the distance. Given a set X of n points and a distance function, k-nearest neighbor (kNN) search lets you find the k closest points in X to a query point or set of points. kNN-based algorithms are widely used as benchmark ML rules.

\textbf{Ensemble classifiers:} Combine results from many weak classifiers into one high-quality ensemble model. Qualities depend on the choice of algorithm. All ensemble classifiers tend to be slow to fit because they often need many learners.

%\subsection{Original Image}	\label{app:gundi}
%The original, unmodified cat image used to visualize the adversarial learning attacks is shown in Figure~\ref{appfig:gundi}.
%
%\begin{figure}[]
%	\centering
%	\includegraphics[width=0.87\columnwidth]{images/gundi_small.jpg}
%	\caption{Original, unmodified cat image used to visualize the adversarial learning attacks.}
%	\label{appfig:gundi}
%\end{figure}

\subsection{List of the Profiled Applications}\label{app:test_classes}

The following is the full list of applications used as the test classes in our experiments.

\begin{enumerate}[noitemsep]
	\item AES-128-CBC
	\item BF-CBC
	\item BLOWFISH
	\item CAMELLIA-128-CBC
	\item DES-CBC
	\item DES-EDE3
	\item DSA2048
	\item ECDH
	\item ECDHB571
	\item ECDHK571
	\item ECDHP521
	\item ECDSA
	\item ECDSAB571
	\item ECDSAP521
	\item HMAC
	\item MD4
	\item MD5
	\item RC2
	\item RC2-CBC
	\item RC4
%	\item rsa2048
%	\item seed
%	\item seed-cbc
%	\item sha1
%	\item sha256
\end{enumerate}

\subsection{CNN Classifier Results}\label{app:class_results}

Here we present the training and validations results of the attacker Eve's application classifier. As seen in the Figure~\ref{appfig:CNN_results_sample}, when the number of samples per class is increased gradually from 100 to 30000, validation accuracy saturates in fewer epochs.

\begin{figure*}[t!]
	\centering
	\includegraphics[width=.95\columnwidth]{images/training/combined/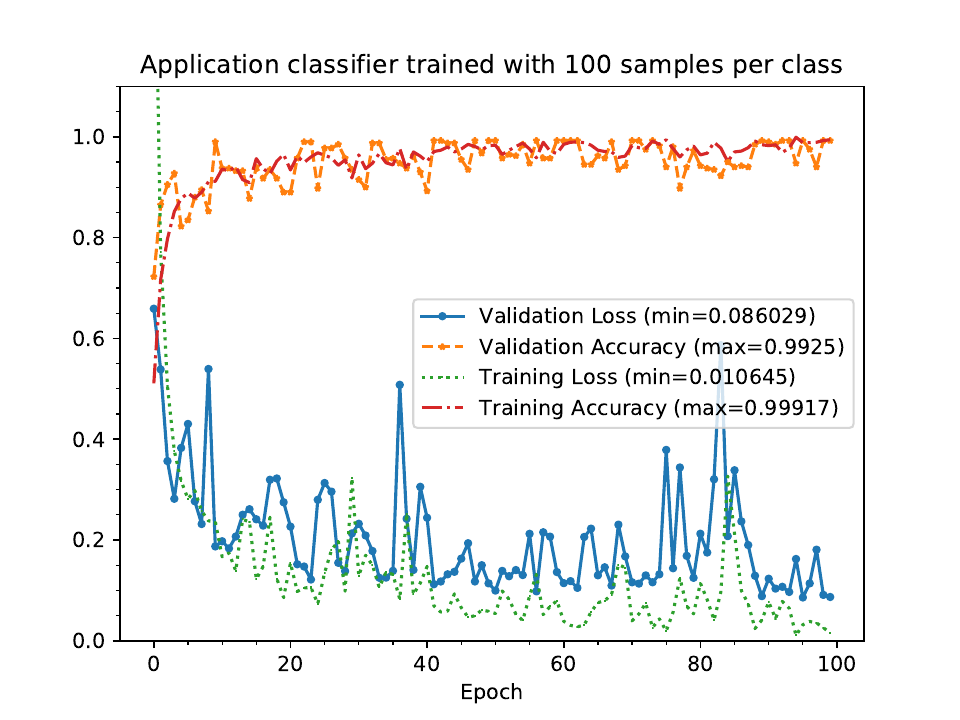}
	\includegraphics[width=.95\columnwidth]{images/training/combined/fig_batch13_c20_s300_f1000_h5_e100.pdf}
	\includegraphics[width=.95\columnwidth]{images/training/combined/fig_batch13-30k_c20_s1000_f1000_h5_e100.pdf}
	\includegraphics[width=.95\columnwidth]{images/training/combined/fig_batch13_c20_s3000_f1000_h5_e100.pdf}
	\includegraphics[width=.95\columnwidth]{images/training/combined/fig_batch13-30k_c20_s10000_f1000_h5_e100.pdf}
	\includegraphics[width=.95\columnwidth]{images/training/combined/fig_batch13-30k_c20_s30000_f1000_h5_e100.pdf}
	\caption{Results of the CNN classifier trained using varying number of samples per class, 100, 300, 1000, 3000 and 10000 in order. As the number of samples increase, number of epochs to achieve high accuracy decreases.}
	\label{appfig:CNN_results_sample}
\end{figure*}

\begin{figure*}[!tb]
	\centering
	\includegraphics[width=.95\columnwidth]{images/training/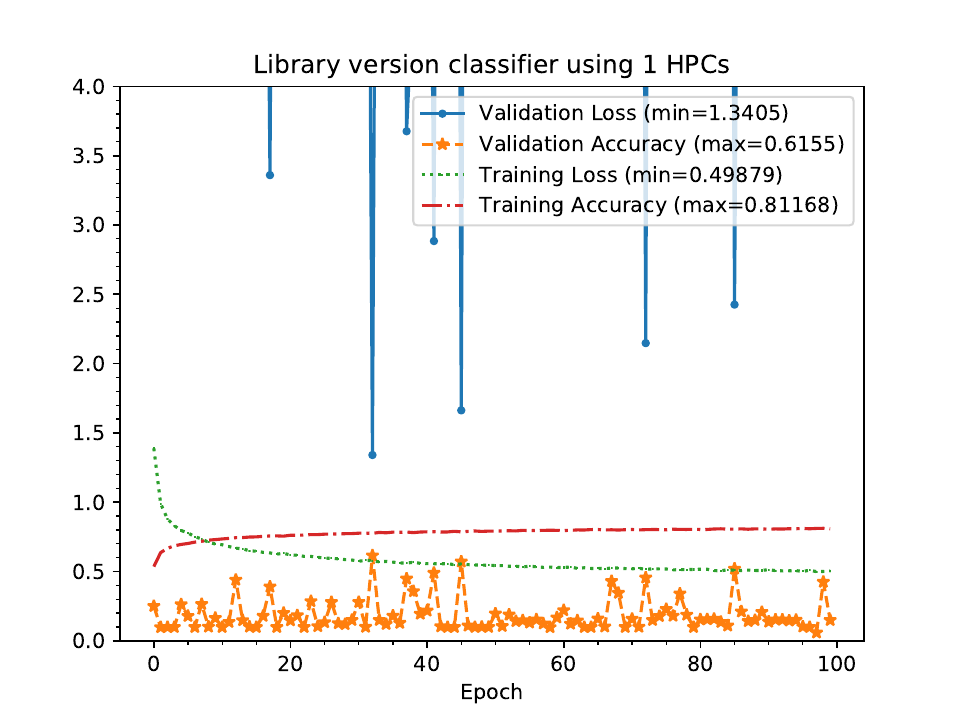}
	\includegraphics[width=.95\columnwidth]{images/training/libhpc2.pdf}
	\includegraphics[width=.95\columnwidth]{images/training/libhpc3.pdf}
	\includegraphics[width=.95\columnwidth]{images/training/libhpc4.pdf}
	\includegraphics[width=.95\columnwidth]{images/training/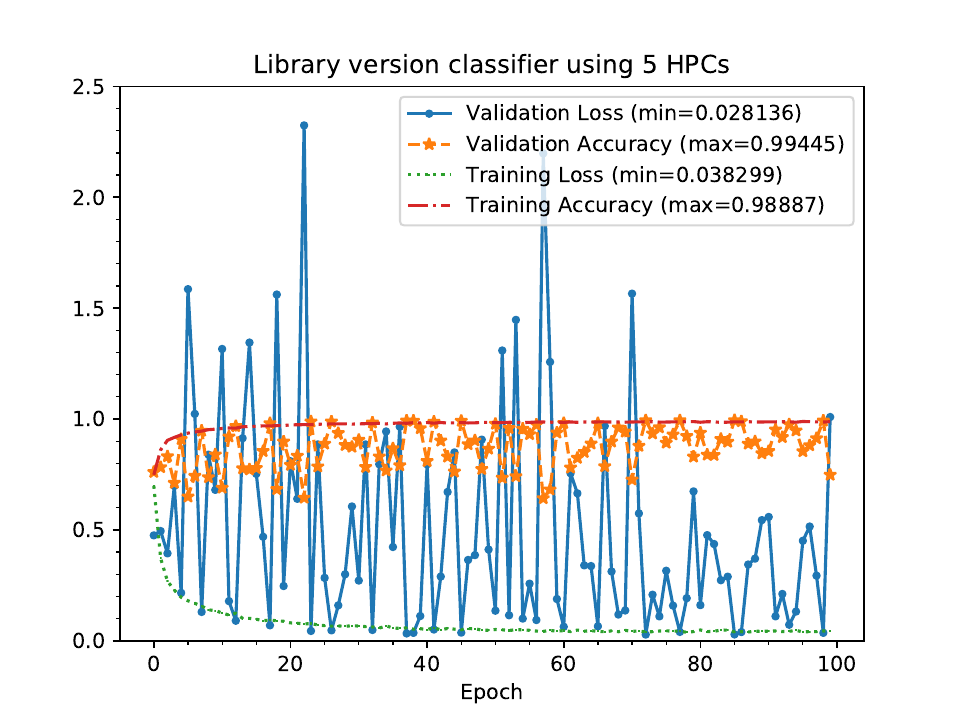}

	\caption{Results of the CNN classifier trained for OpenSSL version detection using varying number of HPCs. When trained with only a single HPC trace, the validation accuracy saturates at 81\%. When more HPCs are used, validation accuracy increases to 99\%.}
	\label{appfig:CNN_results_lib}
\end{figure*}
